# Supplementary material for: A short study comparing countries on the quality of response to the Covid-19 pandemic
Source: arXiv:2109.15055 ancillary file (2022-05-06)
Supplement: Supplementary file 1 [file Supplementary.pdf]

# Supplementary: A short study comparing countries on the quality of response to the Covid-19 pandemic

Thilakam Venkatapathi

*Department of Pathology, University of Kentucky, Lexington, KY 40536*

Murugesan Venkatapathi

*Department of Computational & Data Sciences, Indian Institute of Science, Bangalore 560012*

---

## 1. Methods: A formula for the quality of response to a pandemic

The correlations shown in Figure 1, allow us to ascertain how the positive factors such as vaccine doses ( $V$ ) and the number of tests ( $T$ ) in population-normalized numbers, compare to deaths per million ( $D$ ), given the per capita GDP-PPP ( $G$ ) of a country. Let the corresponding ratios of the negative factors and the positive factors be given by  $F$  below:

$$F = c_0 \frac{\frac{D}{G}}{\sqrt{\frac{V}{G} \cdot \frac{T}{G}}} = c_0 \frac{D}{\sqrt{VT}} \quad (1)$$

where we have used the *geometric* mean given by the square-root of the vaccination and testing rates, to retrieve a value of  $F$  that is independent of the GDP and includes only the main parameters of interest here. The constant  $c_0$  relates the optimal ratio (scaling) of vaccine doses and tests, and estimating it is beyond the scope of this work. Here we set  $c_0$  to 1 without affecting the relative rankings of countries. When the values of  $F$  are used to compare responses to two different pandemics, estimating a specific value for  $c_0$  may become indispensable. In contrast to an arithmetic mean  $(V + T)/2$ , the geometric mean  $\sqrt{VT}$  used also has an implicit inference. It implies that the tests or the vaccinations cannot be easily replaced by the other, and a lower value in one disproportionately reduces effectiveness of the response. While  $F$  in equation 1 used only the idea of correlations, and is a reasonable point to begin with, it requires further additions to increase the robustness of the formula. This can be typically done by considering fundamental conservation properties in the problem. Both, vaccinations to add immunity to the population and the tests performed for breaking the chain in the transmissions, have to be reasonably optimal and finite. Vaccinations contribute effectively to reducing deaths if administered before the majority of the people are exposed to the pathogen, and also the possibility of

---

*Email addresses:* [thilakammur@gmail.com](mailto:thilakammur@gmail.com) (Thilakam Venkatapathi), [muruges@iisc.ac.in](mailto:muruges@iisc.ac.in) (Murugesan Venkatapathi)

partially effective vaccines have to be included. Similarly, testing helps in breaking the chain only if a small fraction of the tests are positive i.e. sufficient number of tests are performed. The above conditions imposed by the problem can be included in evaluating  $F$  as below, using the population-normalized number of confirmed cases  $C$  as well.

$$F = \frac{D}{e^{-(\frac{D}{D_0} + \frac{p}{p_0})} \sqrt{VT}} \text{ where } p = \frac{C}{T} \quad (2)$$

Thus, there are two exponential factors in  $F$  modulating the effectiveness of the vaccinations and tests.  $D_0$  and  $p_0$  representing the *half-life* determine the fully effective regions given by the very small values of  $D$  and  $p$ , and the ineffective regions given by their large values.  $D_0$  represents the potential deaths when all the million people are infected in the absence of vaccines and the treatments available to the patients remain unaltered. Note that large gains in immunity due to the vaccine accrue when most of the population is yet to be infected with the actual pathogen at least once i.e when the deaths  $D \ll D_0$ . Also, a widely used but ineffective vaccine results in the unfortunate eventuality of large deaths  $D \gtrsim D_0$  as has been observed in parts of the world, and thus the above formula takes into account such cases. Similarly, the tests ( $T$ ) are corrected using the known average test positivity ratios  $p$  in  $\exp(-\frac{p}{p_0})$ , for their use in the prevention of transmission. A large positivity ratio  $p$  i.e. larger fraction of positive results  $C$  in the tests  $T$ , implies the tests have been largely used in confirming cases with already strong symptoms. This factor can also be interpreted as a correction factor to the deaths  $D$ , for under-reporting of Covid deaths due to inadequate testing. Other under-recordings of deaths due to varying administrative efficiencies and medical classifications used, cannot be corrected for. But, the lower sensitivity of the rankings due to such uncertainties in the data are shown in the supplementary note. An ideal scoring formula satisfies the basic notions of the problem and produces well distributed scores representing the changes in the input data i.e. it displays adequate sensitivity in the entire range of the input data. On the other hand, it should not exhibit too much sensitivity where the noise in the data dominates the ranking established by the scores.

For our convenience, we can suppress the exponentially varying values of  $F$  without affecting the ordering of the scores or the resulting rankings, by using the log-function.

$$S = \log(1 + FG) \text{ where } F = \frac{a_0 D}{e^{-(\frac{a_0 D}{D_0} + \frac{p}{p_0})} \sqrt{VT}} \quad (3)$$

where  $G$  represents the GDP per capita in PPP terms for the population scored, giving us the units of dollars per vaccine for the evaluated scores. For the *actual* rankings of countries, any constant value of  $G$  and  $a_0$ , like the average per capita values of the world and  $a_0=1$  can be used. This implies that there is no compensation in scores for the varying economic conditions and ages of the population. For a compensated ranking with a hypothetical parity in economic and age factors of the populations, we use a varying  $G$  given by the per capita GDP-PPP of the country, and an  $a_0$  given by the ratio of the fraction of the senior population globally and the fraction of seniors within the country. This leaves us with the values of only the constants  $D_0$  and  $p_0$  to be assigned. As mentioned earlier, the fatality rates are a strong function of the age group, and the measured infection-fatality-rates using sero-surveys have varied from negligible values to 1.2% depending on the age distribution of the sampled population

[1]. The median fatality rates were 0.24%, and we use a value of 0.3% representing the global age distribution to arrive at a  $D_0$  of 3000 deaths per million [1, 2]. Similarly, the maximum value of  $p$  suggested by the World-Health-Organization (WHO) is 0.1 beyond which tests become increasingly useless in breaking chains of transmission, and we use 0.1 as the half life  $p_0$  for tests. Due to this additional exponential term with  $p_0$  and  $D_0$ , low reported deaths due to poor testing rates, or high rates of ineffective vaccines, get notably corrected. This adds to the robustness of the ranking list to noise and unproductive mitigation efforts.

## 2. A study on the ranking list for robustness to noisy data

Ranking problems can be of many kinds; ranking inter-connected objects represented by a graph is the most well-known among them and is used in ranking pages on the world-wide-web [3–5]. The other common problem is the determination of an effective ranking of items when only pair-wise rankings are provided, and this is significant for generating ranking-tables in sports [6]. A third type may involve ranking items based on multiple ranking lists provided [7], representing a market survey for example. Our problem here in studying robustness is more straight-forward and is amenable to a more precise definition. Given a list of countries, a  $n$ -dimensional vector  $\hat{R}$  with natural numbers 1 to  $n$  can be used to represent their rankings. Let  $\Delta\hat{R}$  be the change in the ranking vector due to change in the inputs of the scoring formula. We compensate for the (potential) under-reported deaths depending on the noise levels expected in the data. Similarly, the reported number of tests are expected to be an overestimate of the actual productive tests performed, and hence deflated as well. Note that these are independent errors accrued in countries governed by different institutions and can be represented by random numbers multiplied to the reported data. If data from all the countries included the same level of reporting errors, the rankings do not change and this analysis would be unnecessary. We are interested in evaluating the reliability of the rankings by determining a vector  $\Delta\hat{R}$  that has the *maximum*  $l_1$ -norm, given the magnitude of changes expected in the scores  $F$ . The  $l_1$ -norm  $\|\cdot\|_1$  implies that the length of the vector  $\Delta\hat{R}$  representing the change in ranking list is given by the sum of absolute values of the entries i.e.  $\sum_n |\Delta R_i|$ , and the maximum value of  $\|\Delta\hat{R}\|_1 / n$  is the maximum possible (average) change in the rank of all the  $n$  countries in the list. Note that the simple sum of the signed entries  $\sum_n \Delta R_i$  is always zero as the increase in the rank of a country is always accompanied by an equivalent decrease of ranks of the other countries in the list. Of secondary importance, is determining vectors  $\Delta\hat{R}$  that have the *maximum*  $l_\infty$ -norm i.e. largest absolute value of any entry, representing the *maximum possible* change of rank of *any* country in the list.

Though it is not required for us here, a more formal mathematical statement of the problem is the following. Let the values of evaluated  $F_i$  for all countries  $i$  in the list be given by vector  $\hat{F}$ , and the ordinal ranks (where no two countries share the same rank even if the scores are identical) be given by a function  $f : \mathbb{R}^n \rightarrow \mathbb{N}_1^n$  with  $\|f(\hat{F})\|_1 = \frac{n(n+1)}{2}$ , then we are interested in:

$$\sup_{\Delta\hat{F}_i / \hat{F}_i \in \mathcal{U}(0, e)} \|f(\hat{F}) - f(\hat{F} + \Delta\hat{F})\|_p \quad (4)$$

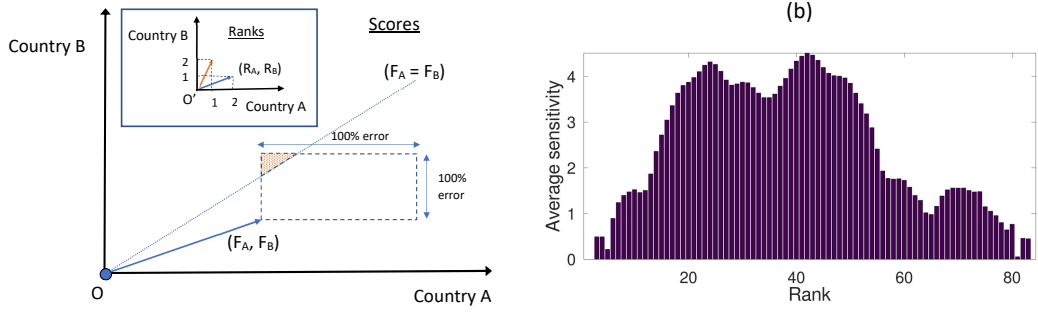

Figure 1: (a) Geometry of the problem explained using scores  $F$  of 2 countries A and B. The rank vector  $\hat{R}$  changes only for the scores given by the shaded triangle where  $F_B > F_A$ , and this becomes a possibility in the presence of errors up to 100% in the data given by all possible scores in the rectangle. When  $n$  countries are in the ranking list, this 2D box changes to an  $n$ -D box ( $n$ -orthotope) with  $2^n$  corners, with largest change of the ranking list given by one of these numerous corners of the box. A random sampling in the box provides the maximum change possible in the ranks with some confidence measure. (b) Average sensitivity reflected by the change in ranking due to 0 – 100% errors at the different original ranks in the list of large countries.

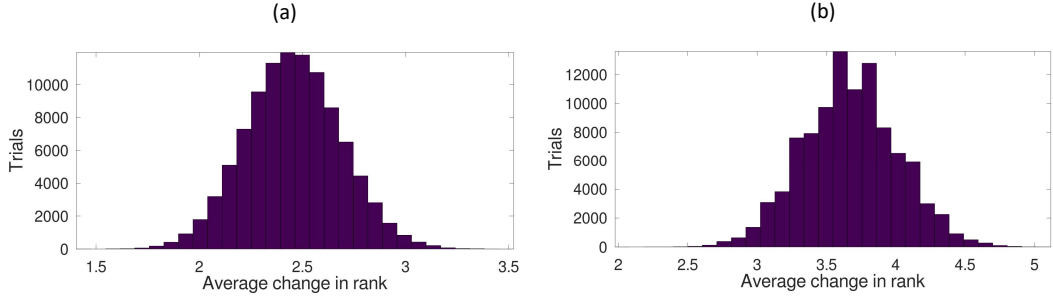

Figure 2: Histograms of average change in the ranks of the list of large countries for  $10^5$  random trials. Ranking list of the smaller countries is even more robust. (a) 0 – 100% errors (b) 0 – 200% errors.

where  $p$  is either 1 or  $\infty$  for the two different norms, and  $e$  in the uniform distribution  $\mathcal{U}$  represents the maximum possible relative error in each entry of  $\hat{F}$ . We study cases where  $e$  is 1 and 2 representing errors up to 100% and errors up to 200% respectively. A geometrical description of the problem and the results of analysis are described in the following figures.

In Figure 1a the rank vector  $\hat{R}$  changes (in the inset) only for the pairs of scores given by the *shaded triangle* where  $F_B > F_A$ , and this becomes a possibility in the presence of errors up to 100% in the data given by all possible scores in the rectangle. When  $n$  countries are in the ranking list, this 2D box changes to an  $n$ -D box ( $n$ -orthotope) with  $2^n$  corners, with largest change of ranks  $\|\Delta\hat{R}\|_1$  given by one of these corners of the box. This maximum possible change of the entire ranking list i.e. maximum average change in ranks, is in general impossible to ascertain analytically, and even computationally when  $n$  is significantly larger than 20 due to the  $2^n$  ranking lists required to be tested. The number of lists to be tested can be significantly reduced by hierarchical algorithms,

but the most effective alternate approach is a random sampling of the possible ranking lists providing the maximum (average) change possible in the ranks with a confidence measure, and this is an approximate solution for eq. (4). This can be done easily using random samples with a uniform probability density in an  $n$ -box defined by the magnitude of errors, which are arbitrarily close to its corners, and such results as presented here may require only  $\sim 2^{17}$  random lists to be generated. Whereas, the maximum possible change in rank for *any* country requires only the  $l_\infty$ -norm i.e.  $\|\Delta\hat{R}\|_\infty$ , and this requires checking the maximum places any country can move if the corresponding error of 100% or 200% is added to the values of all the other  $n - 1$  countries in the list. This is equivalent to checking the ranking lists given by only  $n$  specific corners among the  $2^n$  corners of the box in Figure 1a. This is relatively trivial to do and these values are correspondingly 19 and 28 ranks at most in the list of larger countries, 14 and 19 ranks respectively in the list of smaller countries, for errors up to 100% and 200%. Since these represent the stability of the rank of a single object in the list, they are not as significant as the maximum possible average change in ranks given by  $\|\Delta\hat{R}\|_1/n$ , which is presented in Figure 2 for the noise expected in the data.

## References

- [1] John P. A. Ioannidis. Infection fatality rate of covid-19 inferred from seroprevalence data. *Bull. World Health Organ.*, 99:19–33F, 2021.
- [2] Andrew T. Levin, William P. Hanage, Nana Owusu-Boaitey, Kensington B. Cochran, Seamus P. Walsh, and Gideon Meyerowitz-Katz. Assessing the age specificity of infection fatality rates for covid-19: systematic review, meta-analysis, and public policy implications. *European Journal of Epidemiology*, 35(12):1123–1138, Dec 2020.
- [3] Larry Page, Sergey Brin, R. Motwani, and T. Winograd. The pagerank citation ranking: Bringing order to the web, 1998.
- [4] Huan Sun and Yimin Wei. A note on the pagerank algorithm. *Applied Mathematics and Computation*, 179(2):799–806, 2006.
- [5] Daniel Silvestre, João Hespanha, and Carlos Silvestre. A pagerank algorithm based on asynchronous Gauss-Seidel iterations. In *2018 Annual American Control Conference (ACC)*, pages 484–489, 2018.
- [6] Timothy P. Chartier, Erich Kreutzer, Amy N. Langville, and Kathryn E. Pedings. Sensitivity and stability of ranking vectors. *SIAM Journal on Scientific Computing*, 33(3):1077–1102, 2011.
- [7] Milton Friedman. A Comparison of Alternative Tests of Significance for the Problem of  $m$  Rankings. *The Annals of Mathematical Statistics*, 11(1):86 – 92, 1940.
